# Supplementary material for: When to Memorize and When to Stop: Gated Recurrent Memory for Long-Context Reasoning
Source: arXiv:2602.10560 source file (2026-02-11)
Supplement: Supplementary file 1 [file appendix.tex]

\section{Hello World}
%\subsection{Hello World}
